# Supplementary material for: A Synthetic Modal Generation of Additive Manufacturing Roughness Surfaces from Images
Source: arXiv:2401.01345 source file (2023-10-31)
Supplement: Supplementary file 1 [file Appendix.tex]

\appendix
\section{Derivation of the Rogallo Initialization in \gls{2D}}
\label{sec:RogalloInitiallizationMethod}
In 1981, Rogallo (a \gls{NASA} researcher) derived a mathematical procedure that allows to recreate an initialized isotopic turbulence field (\gls{sym:u}) from an \gls{1D} Energy Spectrum for turbulence flow simulations. A random number generator based on Energy Spectrum is used to create a multidimensional spectral space representation of a velocity field \gls{sym:uhat} that can then be transformed back to physical space using the \gls{IDFT} \cite{Rogallo1981}. The generated synthetic field satisfies: isotropy, continuity and conjugate symmetry in spectral space.

The original mathematical procedure is derived for a \gls{3D} flow field. However, only a \gls{2D} representation is necessary in the case of this internship project. The derivation of the \gls{2D} synthetic turbulence field generation procedure is therefore discussed. However, the derivation contains the same steps as for the \gls{3D} situation. The derivation consists out of two steps. First, the derivation of the Random number generator, which is discussed in \autoref{sec:RandomNumberGenerator}. Secondly, the set-up of the synthetic field using the random number generator, which is presented in \ref{sec:CoordinateTransformation}.

\subsection{Random Number Generator}
\label{sec:RandomNumberGenerator}
To generate a synthetic \gls{2D} (or \gls{3D}) field from a \gls{1D} Energy Spectrum, extra numbers need to be generated to fill this higher dimensional space. This is done by means of random numbers and a random number generator.

To derive an equation for the Random Number Generator \gls{sym:alpha}(\gls{sym:kvectormagnitude}), consider the relation between the \gls{1D} Energy Spectrum (\gls{sym:E}(\gls{sym:kvectormagnitude})) and the trace of the two-point correlation tensor in spectral space $\gls{sym:Rtensorhat}[_{\gls{sub:ii}}]$ given by \autoref{eq:RelationRijEk}), where \gls{sub:ii} is the tensor trace index notation and \gls{sym:sigma} is an integration constant \cite{NieuwstadtEtAl2016}.
\begin{equation}
\label{eq:RelationRijEk}
    E(|\mathbf{k}|) = \frac{1}{2} \oint_{|\mathbf{k}|} \hat{\mathbf{R}}_{ii}(k) d\sigma
\end{equation}
This equation describes that the energy spectrum in a two-point correlated field is defined by integrating the two-point correlation tensor in spectral space over \gls{2D} rings with a radius equal to the magnitude of the wave vector (\gls{sym:kvectormagnitude}). Just like with the definition of the energy spectrum as described in \autoref{sec:EnergySpectrum}. 
The integral over the ring simplifies to the circumference of the ring ($2 \pi \gls{sym:kvectormagnitude}$):
\begin{equation*}
     E(|\mathbf{k}|) = \frac{1}{2} \hat{\mathbf{R}}_{ii}(\mathbf{k}) 2 \pi |\mathbf{k}| = \hat{\mathbf{R}}_{ii}(k) \pi |\mathbf{k}|.
\end{equation*}
After some rearranging, an expression for the two-point correlation tensor is found as shown in \autoref{eq:RNGmagnitude}. 
\begin{equation}
\label{eq:RNGmagnitude}
\begin{split}
    \hat{\mathbf{R}}_{ii}(k) = \frac{E(|\mathbf{k}|)}{\pi |\mathbf{k}|}
\end{split}
\end{equation}

The two-point correlation tensor in spectral space ($\gls{sym:Rtensorhat}[_{\gls{sub:ij}}]$) needs to be conjugate symmetric for it to yield a zero-imaginary part when transformed back into physical space. This is mathematically expressed by \autoref{eq:SymmetryCondition} for a velocity field matrix in spectral space (\gls{sym:uhat}) \cite{NieuwstadtEtAl2016}. Where the bar notation indicates the average and \gls{sub:iindex}, \gls{sub:jindex} are the index notation for the \gls{sym:x} and \gls{sym:y} tensor direction.
\begin{equation}
\label{eq:SymmetryCondition}
    \hat{\mathbf{R}}_{ij} (k) = \overline{\hat{u}^{*}_j (k) \hat{u}_i} (k)
\end{equation}
When combining \autoref{eq:RNGmagnitude} and \ref{eq:SymmetryCondition}, a Random Number Generator function $\gls{sym:alpha}\left(\gls{sym:kvectormagnitude}\right)$ can be defined that satisfies the condition:
\begin{equation*}
\label{eq:WeakRNGcondition}
    \hat{\mathbf{R}}_{ii}(k) = \frac{E(|\mathbf{k}|)}{\pi |\mathbf{k}|} = \overline{\alpha \alpha^*}.
\end{equation*}
For the sake of easy implementation, the condition is strengthened by removing the average aspect, resulting in \autoref{eq:StrongRNGcondition}.
\begin{equation}
\label{eq:StrongRNGcondition}
    \hat{\mathbf{R}}_{ii}(k) = \frac{E(|\mathbf{k}|)}{\pi |\mathbf{k}|} = \alpha \alpha^*
\end{equation}

A Random Number Generator function is defined by \autoref{eq:RandomNumberGenerator}, which satisfies \autoref{eq:StrongRNGcondition} and has the Energy Spectrum as an input. Note that \gls{sym:theta} and \gls{sym:Phi} are random numbers. 
\begin{equation}
\label{eq:RandomNumberGenerator}
\begin{split}
    \alpha \left(|\mathbf{k}|\right) = \sqrt{\frac{E\left(|\mathbf{k}|\right)}{\pi |\mathbf{k}|}} e^{\underline{i}\theta} \text{cos} \Phi\\
    \theta \in [-\pi, \pi); \theta \in \mathbb{R}\\
    \Phi \in [0, 2 \pi); \Phi \in \mathbb{R}
\end{split}
\end{equation}

\subsection{Synthetic Turbulence Field}
\label{sec:CoordinateTransformation}
The \gls{2D} synthetic turbulence field is built up using the Random Number Generator from \autoref{sec:RandomNumberGenerator}. This section covers the derivation of the synthetic turbulence field. The derivation starts from the continuity in spectral space: 
\begin{equation*}
    \mathbf{k} \cdot \hat{u} = 0.
\end{equation*}
This equation expresses that that the dot product of the wave number vector \gls{sym:kvector} and the spectral space velocity field \gls{sym:uhat} is equal to zero, meaning that \gls{sym:uhat} is orthogonal to \gls{sym:kvector}. In other words, there is no component of \gls{sym:uhat} that points in the direction of the wave vector \gls{sym:kvector}. Since \gls{sym:kvector} lies in the $\gls{sym:k}[_{\gls{sub:n}}] \gls{sym:k}[_{\gls{sub:m}}]$-plane, \gls{sym:uhat} will have no component in the $\gls{sym:k}[_{\gls{sub:n}}] \gls{sym:k}[_{\gls{sub:m}}]$-plane.

A spectral unit vector basis $\gls{sym:evector}[_{\gls{sub:n}\gls{sub:m}}]$ in the $\gls{sym:k}[_{\gls{sub:n}}] \gls{sym:k}[_{\gls{sub:m}}]$-plane is chosen such that it has its \gls{sym:y}-component $\gls{sym:evector}[_{\gls{sub:m}}]$ aligned with the wave vector \gls{sym:kvector}. This spectral unit vector basis will thus only have a synthetic field in the direction of the $\gls{sym:evector}[_{\gls{sub:n}}]$-direction, see \autoref{fig:RogalloSpectralSpace}.
The synthetic velocity field in spectral space \gls{sym:uhat} should thus only be built using the Random Number Generator in the $\gls{sym:evector}[_{\gls{sub:n}}]$-direction as expressed by \autoref{eq:SyntheticFieldenm}.
\begin{equation}
\label{eq:SyntheticFieldenm}
    \hat{u}_{nm} = \hat{u}\left(k_n, k_m\right) = \alpha \left(|\mathbf{k}|\right) \mathbf{e}_n + 0 \mathbf{e}_m = \begin{bmatrix}
        \alpha \left(|\mathbf{k}|\right) \\ 0
    \end{bmatrix}
\end{equation}
To be able to generate the synthetic field in the $\gls{sym:kvector}[_{\gls{sub:n}}]$$\gls{sym:kvector}[_{\gls{sub:m}}]$-plane, \autoref{eq:SyntheticFieldenm} needs to be transformed to a computational unit vector basis $\gls{sym:bvector}[_{\gls{sub:n}\gls{sub:m}}]$ that has its components $\gls{sym:bvector}[_{\gls{sub:n}}]$ and $\gls{sym:bvector}[_{\gls{sub:m}}]$ aligned with the wave vector components $\gls{sym:kvector}[_{\gls{sub:n}}]$ and $\gls{sym:kvector}[_{\gls{sub:m}}]$ respectively, as shown in \autoref{fig:RogalloSpectralSpace}. 
\begin{figure}[h!]
    \centering
    \includesvg[width=0.8\textwidth]{Images/RogalloFigure.svg}
    \caption{A schematic of the \gls{2D} spectral space velocity field representation \gls{sym:uhat} of the physical space turbulence velocity field \gls{sym:u}, with the Energy Spectrum extraction rings (blue) with a radius \gls{sym:kvectormagnitude}, the spectral unit vector basis components $\gls{sym:evector}[_{\gls{sub:n}}]$ and $\gls{sym:evector}[_{\gls{sub:m}}]$ (green) and the computational unit vector basis components $\gls{sym:bvector}[_{\gls{sub:n}}]$ and $\gls{sym:bvector}[_{\gls{sub:m}}]$ (magenta).}
    \label{fig:RogalloSpectralSpace}
\end{figure}
The computational unit vector basis in the $\gls{sym:kvector}[_{\gls{sub:n}}]\gls{sym:kvector}[_{\gls{sub:m}}]$-plane has the form:
\begin{equation*}
    \mathbf{b}_{nm} = \begin{bmatrix}
        \mathbf{b}_n \\ \mathbf{b}_m
    \end{bmatrix} = \begin{bmatrix}
        1 & 0\\ 0 & 1
    \end{bmatrix} = \mathbf{I}.
\end{equation*}

To be able to find a transformation matrix $\gls{sym:T}[_{\gls{sub:be}}]$ to transform \autoref{eq:SyntheticFieldenm} from the spectral basis to the computational unit basis, an expression is required for the spectral unit vector basis $\gls{sym:evector}[_{\gls{sub:n}\gls{sub:m}}]$. Since the $\gls{sym:evector}[_{\gls{sub:m}}]$-component is aligned with \gls{sym:kvectormagnitude}, $\gls{sym:evector}[_{\gls{sub:m}}]$ can be expressed as:
\begin{equation*}
    \mathbf{e}_m = \begin{bmatrix}
        \frac{\mathbf{k}_n}{|\mathbf{k}|} \\ \frac{\mathbf{k}_m}{|\mathbf{k}|}
    \end{bmatrix},
\end{equation*}
where each component is normalized with the magnitude of the wave vector to create a unit vector basis.

The $\gls{sym:evector}[_{\gls{sub:n}}]$ component can be found be realizing that it needs to be orthogonal to $\gls{sym:evector}[_{\gls{sub:m}}]$ to form a vector basis. For now, the unknown component $\gls{sym:evector}[_{\gls{sub:n}}]$ is expressed as:
\begin{equation*}
\begin{split}
    \mathbf{e}_n = \begin{bmatrix}
        \frac{\mathbf{e}_{n_{0}}}{|\mathbf{e}_n|} \\ 
        \frac{\mathbf{e}_{n_{1}}}{|\mathbf{e}_n|}
    \end{bmatrix},
\end{split}
\end{equation*}
Using the definition of the dot product, it follows that:
\begin{equation*}
\begin{split}
    \mathbf{e}_n \cdot \mathbf{e}_m &= 0, \\
     \begin{bmatrix}
        \frac{\mathbf{e}_{n_{0}}}{|\mathbf{e}_n|} \\ \frac{\mathbf{e}_{n_{1}}}{|\mathbf{e}_n|}
    \end{bmatrix} \cdot \begin{bmatrix}
        \frac{\mathbf{k}_n}{|\mathbf{k}|} \\ \frac{\mathbf{k}_m}{|\mathbf{k}|}
    \end{bmatrix} &= 0, \\
    \frac{\mathbf{e}_{n_{0}}\mathbf{k}_n}{|\mathbf{e}_n||\mathbf{k}|} + \frac{\mathbf{e}_{n_{1}}\mathbf{k}_m}{|\mathbf{e}_n||\mathbf{k}|} &= 0, \\
    \mathbf{e}_{n_{0}}\mathbf{k}_n + \mathbf{e}_{n_{1}}\mathbf{k}_m &= 0.
\end{split}
\end{equation*}
It can thus be concluded that $\gls{sym:evector}[_{\gls{sub:n}_{0}}] = \gls{sym:kvector}[_{\gls{sub:m}}]$, $\gls{sym:evector}[_{\gls{sub:n}_{1}}] = -\gls{sym:kvector}[_{\gls{sub:n}}]$, resulting in $|\gls{sym:evector}[_{\gls{sub:n}}]| = \gls{sym:kvectormagnitude}$. The following expression is found for the computational unit vector basis:
\begin{equation*}
    \mathbf{e}_{nm} = \begin{bmatrix}
        \mathbf{e}_n \\ \mathbf{e}_m
    \end{bmatrix} = 
    \begin{bmatrix}
        \frac{\mathbf{k}_m}{|\mathbf{k}|} & -\frac{\mathbf{k}_n}{|\mathbf{k}|} \\
        \frac{\mathbf{k}_n}{|\mathbf{k}|} & \frac{\mathbf{k}_m}{|\mathbf{k}|}
    \end{bmatrix}.
\end{equation*}
To get an expression for the transformation matrix $\gls{sym:T}[_{\gls{sub:be}}]$ one needs to realize that $\gls{sym:bvector}[_{\gls{sub:n}\gls{sub:m}}]$ and $\gls{sym:evector}[_{\gls{sub:n}\gls{sub:m}}]$ are both orthogonal matrices, meaning that their inverse is equal to their transpose. Also, $\gls{sym:bvector}[_{\gls{sub:n}\gls{sub:m}}]$ is equal to the identity matrix \gls{sym:identity}. To transform from $\gls{sym:evector}[_{\gls{sub:n}\gls{sub:m}}]$ to $\gls{sym:bvector}[_{\gls{sub:n}\gls{sub:m}}]$ using $\gls{sym:T}[_{\gls{sub:be}}]$, the following transformation is defined. Both sides are multiplied with the inverse of $\gls{sym:evector}[_{\gls{sub:n}\gls{sub:m}}]$ ($\gls{sym:evector}[^{\gls{sup:inverse}}_{\gls{sub:n}\gls{sub:m}}] = \gls{sym:evector}[^{\gls{sup:transpose}}_{\gls{sub:n}\gls{sub:m}}]$), simplifying results in:
\begin{equation*}
\begin{split}
    \mathbf{b}_{nm} &= \mathbf{T}_{be} \mathbf{e}_{nm}, \\
    \mathbf{e}^{-1}_{nm} \mathbf{b}_{nm} &= \mathbf{e}^{-1}_{nm}\mathbf{T}_{be} \mathbf{e}_{nm}, \\
    \mathbf{e}^{T}_{nm} \mathbf{I} &= \mathbf{T}_{be} \mathbf{I}, \\
    \mathbf{T}_{be} &= \mathbf{e}^{T}_{nm}.
\end{split}
\end{equation*}

When transforming \autoref{eq:SyntheticFieldenm} to the $\gls{sym:bvector}[_{\gls{sub:n}\gls{sub:m}}]$ unit vector basis using $\gls{sym:T}[_{\gls{sub:be}}]$, one finds an expression for the synthetic turbulence velocity field in spectral space $\gls{sym:uhat}[_{\gls{sub:n}\gls{sub:m}}]$, that has the components $\gls{sym:uhat}[_{\gls{sub:n}}]$ and $\gls{sym:uhat}[_{\gls{sub:m}}]$, given by \autoref{eq:SyntheticField2D}.
\begin{equation}
\begin{split}
\label{eq:SyntheticField2D}
    \hat{u}_{nm} = \hat{u} \left(k_n, k_m\right) = \begin{bmatrix}
        \hat{u}_{n} \\ \hat{u}_{m}
    \end{bmatrix} = 
    \begin{bmatrix}
        \hat{u}_n \left(k_n, k_m\right) \\ \hat{u}_m \left(k_n, k_m\right)
    \end{bmatrix} = 
    \begin{bmatrix}
        \alpha \left(|\mathbf{k}|\right) \frac{\mathbf{k}_m}{|\mathbf{k}|} \\ - \alpha \left(|\mathbf{k}|\right) \frac{\mathbf{k}_n}{|\mathbf{k}|}
    \end{bmatrix}; \\
    \hat{u}_{nm}, \hat{u}_{n}, \hat{u}_{m} \in \mathbb{C}^{M \times N}
\end{split}
\end{equation}

The same \autoref{eq:SyntheticField2D} can be obtained from the \gls{3D} equations derived by Rogallo \cite{Rogallo1981} by realizing that in \gls{2D} there is no component in the z-direction, resulting in those terms dropping out. The \gls{3D} equation for the synthetic turbulence field simplifies to \autoref{eq:SyntheticField2D}.
